# Supplementary material for: Mixed eldfellite compounds \ce{Na(Fe_{1/2}M_{1/2})(SO4)2} (M = Mn, Co, Ni): A new family of high electrode potential cathodes for the sodium-ion battery
Source: arXiv:1709.05523 source file (2017-09-16)
Supplement: Supplementary file 1 [file modeldfellite-supp.pdf]

# Supporting information – Design of mixing eldfellite compounds $Na(Fe_{1/2}M_{1/2})(SO_4)_2$ (M = Mn, Co, Ni) with high electrode voltage for sodium-ion battery cathode

Gum-Chol Ri, Song-Hyok Choe, Chol-Jun Yu*

*Department of Computational Materials Design, Faculty of Materials Science, Kim Il Sung University, Ryongnam-Dong, Taesong District, Pyongyang, Democratic People's Republic of Korea*

*Corresponding author: Chol-Jun Yu, ryongnam14@yahoo.com

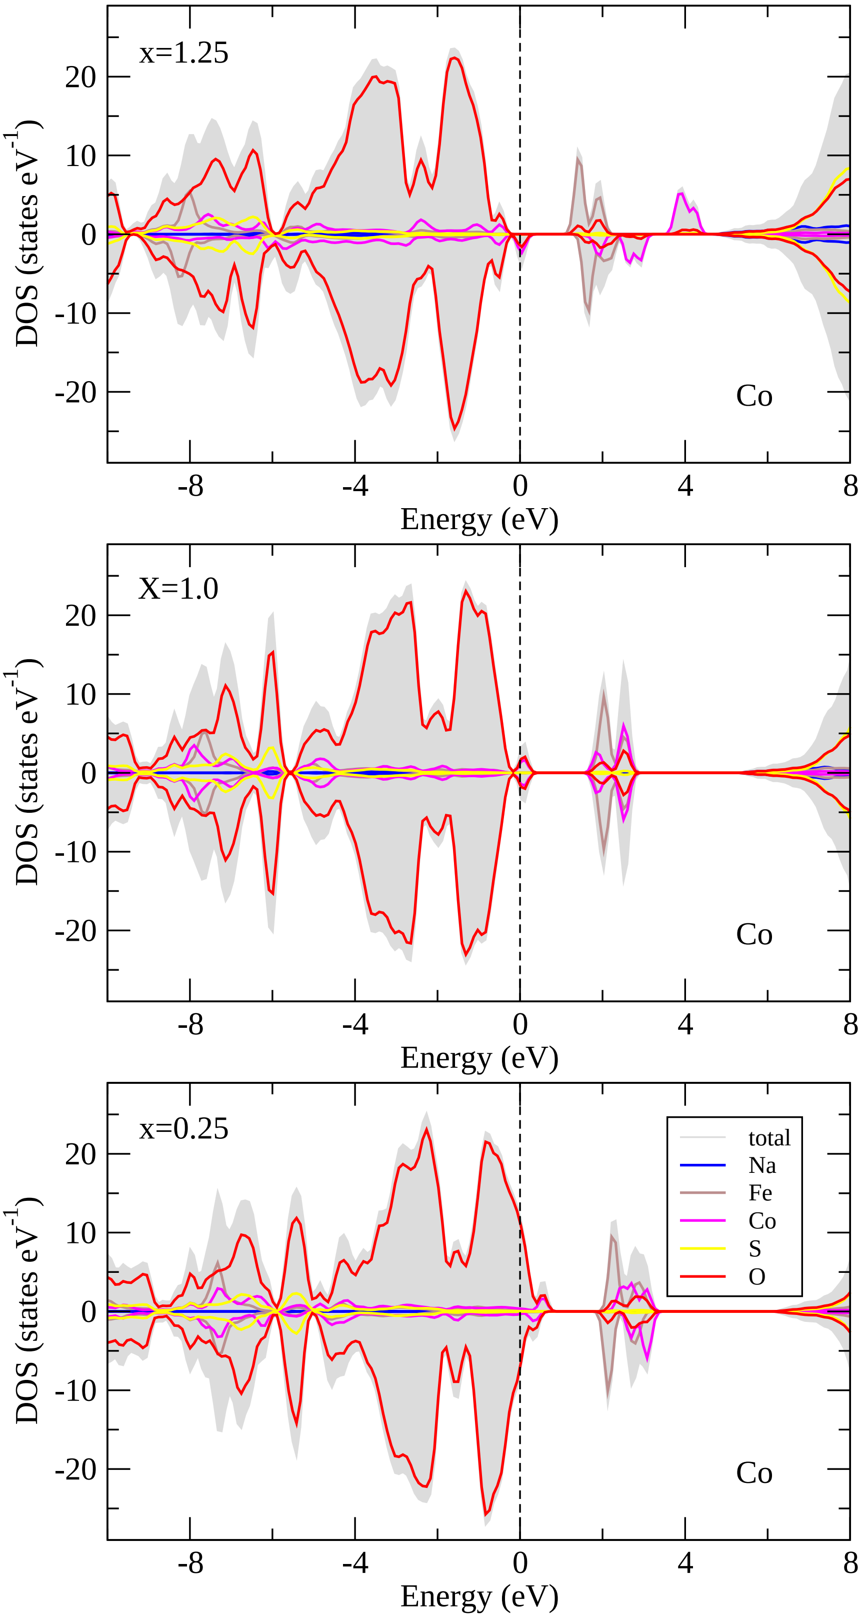


Figure 1: DOS of $Na_x(Fe_{1/2}Co_{1/2})(SO_4)_2$ at x = 0.25, 1.0, 1.25. The Fermi level is set to zero eV.

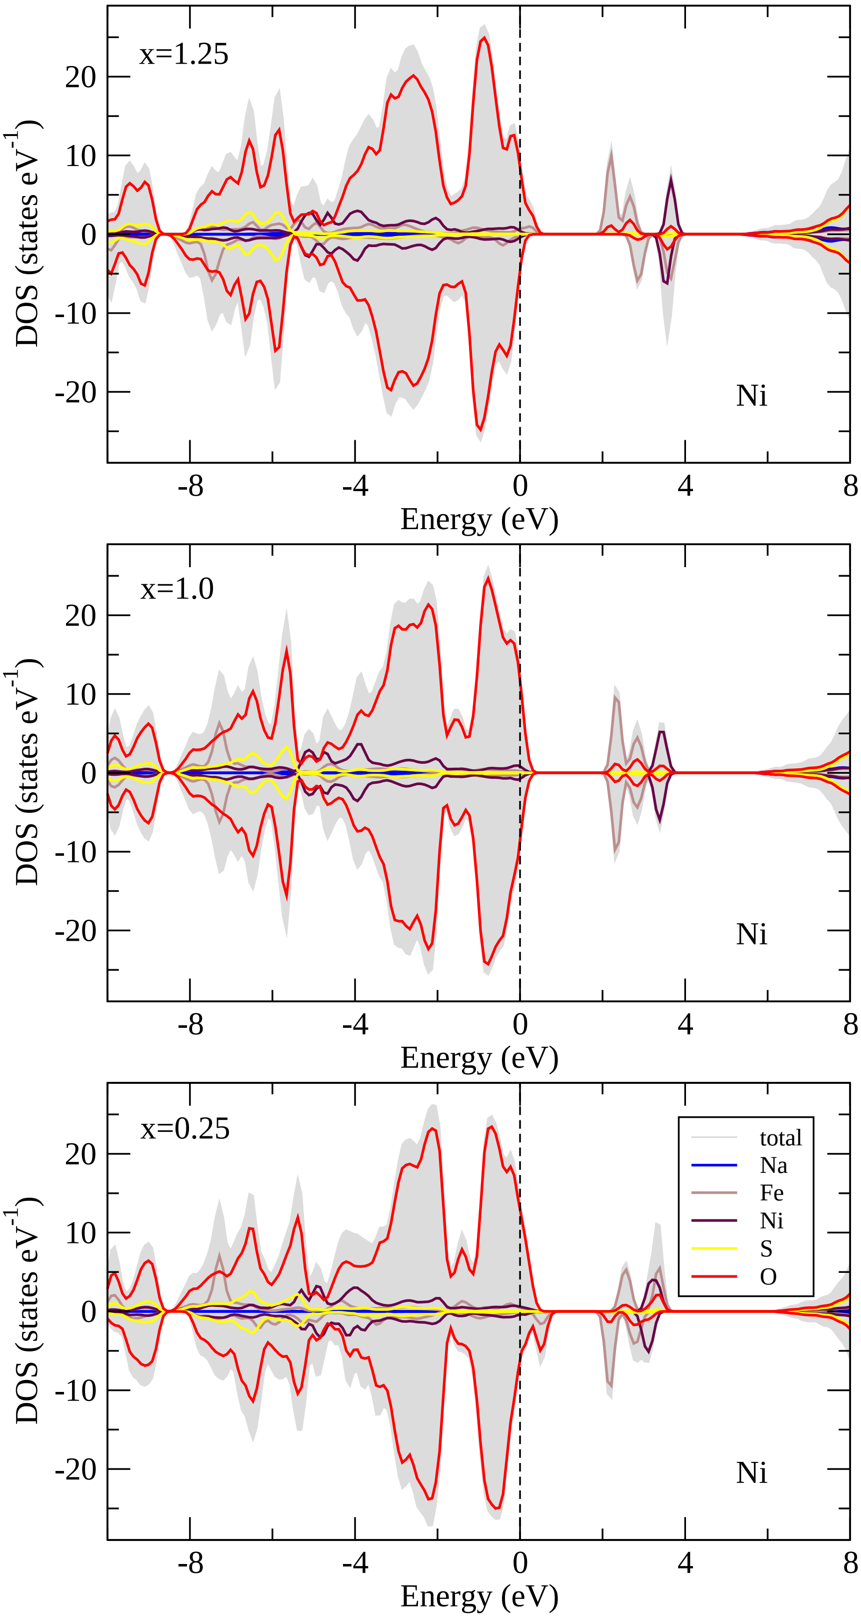


Figure 2: DOS of $Na_x(Fe_{1/2}Ni_{1/2})(SO_4)_2$ at x = 0.25, 1.0, 1.25. The Fermi level is set to zero eV.

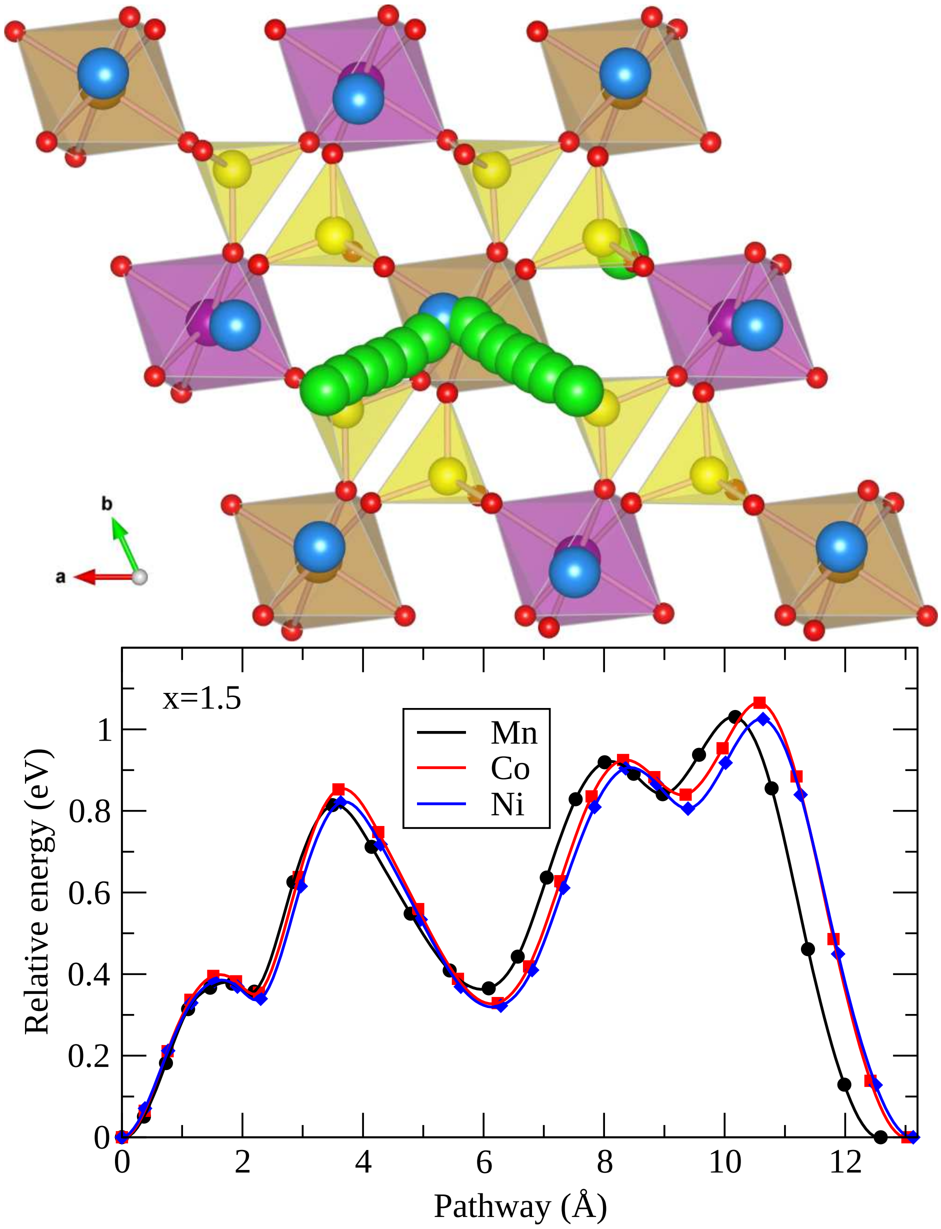


Figure 3: Migration pathway and energy profile for $Na_x(Fe_{1/2}M_{1/2})(SO_4)_2$ (M = Mn, Co, Ni) compounds at x = 1.5.

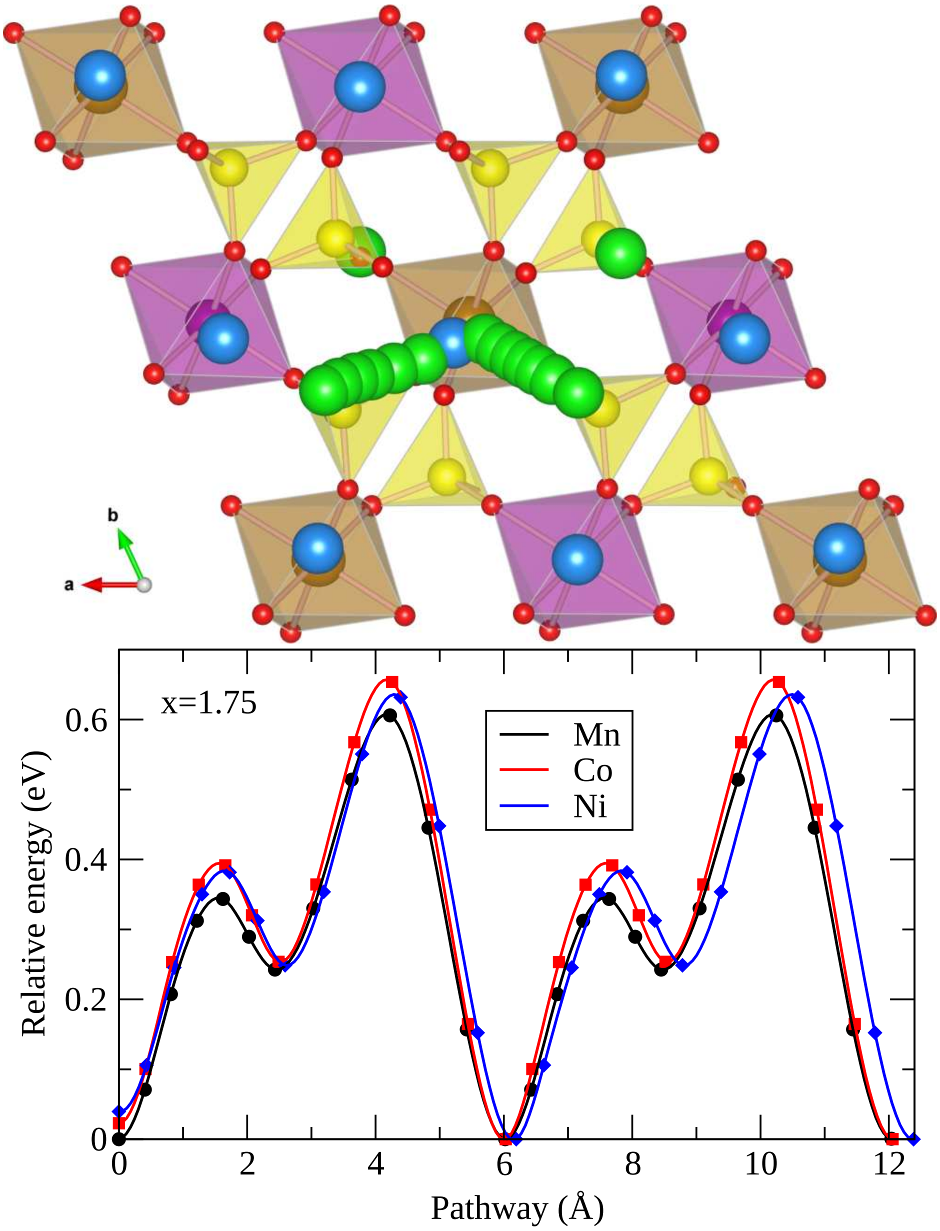


Figure 4: Migration pathway and energy profile for $Na_x(Fe_{1/2}M_{1/2})(SO_4)_2$ (M = Mn, Co, Ni) compounds at x = 1.75.
